# Supplementary material for: Improving and Expanding Video Editing Capabilities Without Videos
Source: arXiv:2611.34941 source file (2026-11-25)
Supplement: Supplementary file 1 [file A_appendix.tex]

\section{Discussion}
\label{app:discussion}

\subsection{Relation to Other Work}
\label{app:relation}

Three lines of work are closest to \methodname: video editors trained from image pairs instead of videos, editors trained without edited targets, and on-policy distillation from image models into video models.

\paragraph{Video Editing from Image Pairs.}
ViFeEdit~\citep{yu2026vifeedit} and ImVideoEdit~\citep{xu2026imvideoedit} also learn video editing without video data. Both build a new video editor from the text-to-video model Wan2.1-T2V-1.3B by adding spatial attention modules, keeping the pretrained 3D attention frozen, and fine-tuning on synthetic image-edit pairs treated as single-frame videos, with edited targets rendered in advance by an image editor. \methodname differs from them in three ways. First, instead of building a new editor from a text-to-video model, \textbf{we keep the architecture unchanged and strengthen existing instruction-based video editors} with a LoRA. Second, \textbf{we need no edited targets} because an existing frozen image editor acts as the teacher and supervises the student's own denoising rollout at every step. Third, while both works evaluate only appearance edits (style, replacement, color, addition, and removal, plus relighting and background replacement in ImVideoEdit) on their own test sets, \textbf{we extend editing to action, expression, and body-movement edits}. Because these edits change how a subject moves across frames, they demand strong temporal consistency, and we show that the temporal quality of the edited videos stays on par with that of the base editors (\Cref{tab:vbench_openvepp,tab:ivebench_main}). We do not compare with ViFeEdit or ImVideoEdit directly, since ImVideoEdit released no code and ViFeEdit released code without trained weights.

\paragraph{Editors Trained without Edited Targets.}
EVE~\citep{singer2024eve} also trains a video editor without supervised video data, building it from a text-to-image model and distilling from two adapters on that model, an image-editing adapter for per-frame edits and a video-generation adapter for temporal consistency. In contrast, we strengthen an existing video editor without changing its architecture, \textbf{using a single frozen image editor and no second teacher}, and temporal quality still stays on par with the base editors. BYG~\citep{tewel2026byg} uses no external teacher at all and trains flow-matching editors without paired examples from the frozen base model's own instruction-following cues and cycle consistency, whereas \textbf{our external image editor can also teach edits that the base video editor does not yet make well}, such as edits that change how a subject moves. UIP2P~\citep{simsar2024uip2p} and NP-Edit~\citep{kumari2025nopairs} also train editors without edited targets, though they work only on images.

\paragraph{On-Policy Distillation from Image Models.}
MILD~\citep{jiang2026mild} improves text-to-video generation with image experts for composition, aesthetics, and text rendering. Its student rolls out whole videos, and the image experts supervise slices of the video latents along that rollout. Because its image and video models use different VAEs, MILD learns connectors to map those slices into the image latent space, anchors the transferred corrections to a frozen copy of the video model, and adds an optical-flow motion reward. In contrast, \methodname \textbf{rolls out single images}: our video editor role-plays as an image editor and edits each source image as a one-frame video, the same input the image editor receives. Since the teacher and the students share a VAE latent space, we need no connectors, and training renders no multi-frame videos.

\subsection{Constructing Paired Video Edits}
\label{app:video_data}

\paragraph{Why Paired Video Edits Are Hard to Build.}
An editing pair needs a source video and a second video that differs from it only in the requested edit.
Such pairs almost never occur naturally~\citep{cheng2024insv2v,pan2026nova}, so existing datasets synthesize them at a high cost~\citep{bai2026ditto} and mostly for appearance edits such as addition, removal, replacement, and style~\citep{he2025openve,burgert2026motionv2v}.
Motion edits are harder still, because the target must change how a subject moves while the rest of the scene, the camera, and the timing follow the source.

\paragraph{Editing One Frame and Regenerating the Video.}
A common shortcut edits one frame with an image editor and lets an image-to-video model generate the rest~\citep{ku2024anyv2v,ouyang2024i2vedit}.
These methods steer the image-to-video model with inverted source features~\citep{ku2024anyv2v} or per-video motion LoRAs~\citep{ouyang2024i2vedit}, and where this guidance is weak, the model regenerates the motion instead of keeping the source motion.
Content that is not visible in the first frame is hallucinated~\citep{burgert2026motionv2v}, the result drifts from the source dynamics under camera or object motion~\citep{pan2026nova}, and the quality of each pair is capped by the propagation model~\citep{bai2026ditto}.
Goku~\citep{liang2026goku} builds part of its \textit{Subject Movement} data in this way: an image editor moves the subject in the first frame, and a video model generates the clip from it.
For action changes, the same video model generates both the source and the target from two text descriptions, so the source is itself synthetic, which transfers poorly to real videos~\citep{wu2025insvie}.
Its filter discards about 88\% of the generated samples, yet the released targets still do not follow the source motion (\Cref{fig:goku_pairs}). Asked to lower a waving hand, the target lowers it and then freezes the person, and asked to turn the torso by 20 degrees, it replaces the whole dance.
\methodname builds no video targets: the student learns from single images and relies on the pretrained video editor for motion.

\begin{figure}[!htb]
\centering
\includegraphics[width=\linewidth]{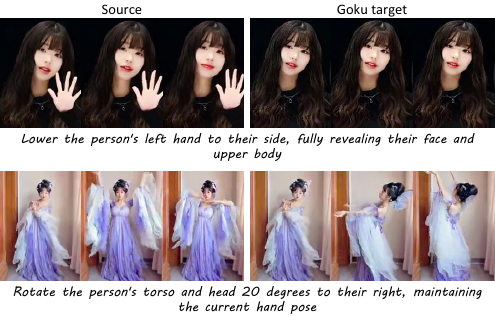}
\caption{\textbf{Released Goku \textit{Subject Movement} pairs.} Top: the target lowers the hand, and the lips that move in the source stay still in the target. Bottom: the target turns the torso and performs a different dance.}
\label{fig:goku_pairs}
\end{figure}

\section{Implementation Details}
\label{app:impl}

\begin{algorithm}[!h]
\caption{One training step of \methodname}
\label{alg:opd}
\begin{algorithmic}[1]
\STATE Sample $(I_s, c_{\mathrm{img}}, c_{\mathrm{video}})$ from the source-only data
\STATE Encode $I_s$ as a one-frame source
\STATE $\vx_{t_K}\gets\epsilon\sim\mathcal{N}(0,I)$, \ $\cL_{\mathrm{I2VT}}\gets 0$
\FOR{$k = K$ \textbf{down to} $1$}
  \STATE $\vv^R_k \gets \theta^{\omega_R}(\vx_{t_k},t_k,c_{\mathrm{video}})$ on all generated frames
  \STATE $\vv^S_k \gets \theta^{\omega_S}(\vx_{t_k},t_k,c_{\mathrm{video}})$ on the edited frame
  \STATE $\vv^T_k \gets \phi^{\omega_T}(\vx_{t_k},t_k,c_{\mathrm{img}})$ on the edited frame
  \STATE $\cL_{\mathrm{I2VT}} \gets \cL_{\mathrm{I2VT}}+\frac{1}{K}\lVert \vv^S_k-\sg(\vv^T_k)\rVert_2^2$
  \STATE $\vx_{t_{k-1}} \gets \sg\bigl(\vx_{t_k}+(t_{k-1}-t_k)\,\vv^R_k\bigr)$
\ENDFOR
\STATE Update the student LoRA with $\nabla_\theta\cL_{\mathrm{I2VT}}$, keeping the image editor $\phi$ frozen
\end{algorithmic}
\end{algorithm}

\paragraph{Bernini-R.}
Bernini-R~\citep{bernini2026bernini} adopts the Wan architecture~\citep{wan2025wan}, including the Wan VAE and the UMT5 text encoder.
Bernini-R-1.3B follows Wan2.1-T2V-1.3B, and Bernini-R-14B follows the two-expert layout of Wan2.2-14B, which denoises high noise levels with one expert and low noise levels with the other.
To edit a video, Bernini-R places the source and target latents in one token sequence and gives the two segments different rotary position embeddings. It reads the instruction through cross-attention and denoises only the target tokens.
At inference, Bernini-R uses adaptive projected guidance (APG)~\citep{sadat2025apg} with separate scales for the source video ($1.25$), the image ($4.5$), and the text ($4.0$).

\paragraph{VideoCoF.}
VideoCoF~\citep{yang2025videocof} adapts Wan2.1-T2V-14B~\citep{wan2025wan} with a LoRA for instruction-based editing without masks.
It arranges the source frames, a reasoning frame, and the edited frames in one sequence along the temporal axis and reads the instruction through cross-attention.
The reasoning frame marks the region to edit, so the model first predicts where to edit and then generates the edited frames.
Its rotary position embeddings align the edited frames with the source frames in time, which keeps the source motion and lets VideoCoF edit videos longer than its training clips. Following its official inference, VideoCoF samples in four steps with the FusionX acceleration LoRA for Wan2.1-T2V-14B~\citep{fusionx2025}.

\paragraph{Training VideoCoF with \methodname.}
The student generates the reasoning and edited frames together, but the loss supervises only the edited frame.
In the loss equations, states and velocities therefore refer to the edited frame, whereas the rollout advances all generated frames.

\paragraph{Solver.}
During each \methodname training step (\Cref{alg:opd}), we use the Euler update with $K=10$ denoising steps on a normalized schedule $1=t_K>\cdots>t_0=0$ and a rollout time shift of $5$ (Appendix~\ref{app:ablation} compares other rollout lengths and time shifts).
At inference, each editor instead uses its official sampler and settings (\Cref{tab:hyperparams}).

\paragraph{Teacher.}
The teacher is JoyAI-Image-Edit~\citep{song2026joyaiimage}, used frozen and without modification.
It receives the image-edit instruction and the student's edited-frame latents and returns a velocity on those latents.
For CFG, the teacher uses an empty instruction and the video student uses its pretrained negative prompt, while both retain the source conditioning.
When $\omega_T>1$, the teacher rescales its guided velocity to the norm of its conditional velocity, as the JoyAI-Image-Edit sampler does.
\begin{figure}[t]
\centering
\includegraphics[width=\linewidth]{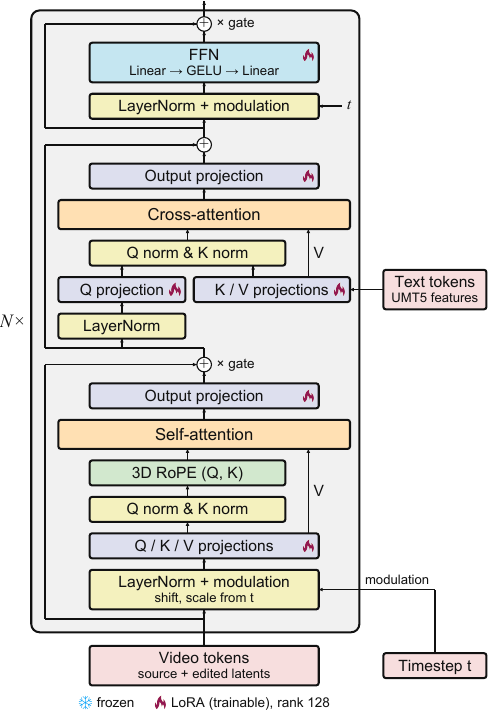}
\caption{\textbf{Transformer block of the student editors.} A rank-128 LoRA trains the linear layers marked with a flame. The block repeats 30 times in Bernini-R-1.3B, 40 times per expert in Bernini-R-14B, and 40 times in VideoCoF.}
\label{fig:wan_block}
\end{figure}

\begin{table*}[t]
\centering
\fontsize{8}{9.5}\selectfont
\setlength{\tabcolsep}{1.6pt}
\begin{tabular*}{\linewidth}{@{\extracolsep{\fill}}>{\hspace{2pt}}llll<{\hspace{2pt}}@{}}
 & \tablehead{Bernini-R-1.3B} & \tablehead{Bernini-R-14B} & \tablehead{VideoCoF} \\
\tabheadrule
\multicolumn{4}{@{}>{\hspace{2pt}}l}{\textbf{Base editor}} \\
Weights & Bernini-R-1.3B & Bernini-R-14B & Wan2.1-T2V-14B + LoRA \\
Edit types & 7 OpenVE categories & 7 OpenVE categories & add, remove, swap, local style \\
\tabbodyrule
\multicolumn{4}{@{}>{\hspace{2pt}}l}{\textbf{\methodname training}} \\
LoRA rank / $\alpha$ & 128 / 64 & 128 / 64 per expert & 128 / 64 \\
Learning rate & $2\times10^{-5}$ & $5\times10^{-5}$ & $5\times10^{-5}$ \\
Effective batch & 24 (joint: 48) & 24 (joint: 48) & 24 (joint: 48) \\
Rollout steps $K$ & 10 & 10 & 10 \\
$\omega_T$ & 1--2$^{\dagger}$ & 1--2$^{\dagger}$ & 2 \\
$\omega_R / \omega_S$ & 1 / 1 & 1 / 1 & 1 / 1 \\
Loss & velocity mse & velocity mse & velocity mse \\
Training steps & 200 & 200 & 200 \\
\tabbodyrule
\multicolumn{4}{@{}>{\hspace{2pt}}l}{\textbf{Inference}} \\
Sampler & UniPC & UniPC & 4-step FusionX LoRA \\
Steps & 40 & 40 & 4 \\
Frames & 81 & 81 & 33 \\
Guidance & APG & APG & none \\
Time shift & 5 & 5 & 5 \\
\end{tabular*}
\caption{\textbf{Editor and training settings.} $^{\dagger}$Both Bernini-R editors use $\omega_T=2$ on actions and body movements and $\omega_T=1$ on the OpenVE pool, expressions, and relighting.}
\label{tab:hyperparams}
\end{table*}

\paragraph{Training Settings.}
We train a LoRA on every linear layer of each student's DiT (\Cref{fig:wan_block}) and keep the backbone frozen. \Cref{tab:hyperparams} lists the settings, and $\omega_R$ and $\omega_S$ stay at $1$ except where \Cref{sec:guidance_scales} varies them.
For VideoCoF, we initialize the editing LoRA from the official VideoCoF LoRA and keep the acceleration LoRA frozen, so the base and fine-tuned editors share it.
Bernini-R-14B uses learning rate $5\times10^{-5}$.
Joint training on \datasetfull takes about 20 A100 GPU-hours for Bernini-R-1.3B on three GPUs and 20--25 B300 GPU-hours for Bernini-R-14B and VideoCoF on two GPUs.
The \modellarge row in \Cref{tab:main} uses one step-200 checkpoint for every benchmark column, with APG guidance $4$, time shift $5$, and seed $42$ at inference.

\paragraph{Two Instructions.}
The image-edit instruction must describe an edit that makes sense for a single image, while the video-edit instruction may mention temporal consistency.
Feeding the video-edit instruction to the teacher, or the image-edit instruction to the student, puts one of the two models outside the input distribution it was trained on.

\section{Training Data Construction}
\label{app:data}

We build two training pools, the OpenVE pool and the \benchname pool (\Cref{tab:pools}). Their union, \datasetfull, trains \modelsmall, \modellarge, and \modelcof in \Cref{tab:main}.
Both pools are \emph{source-only}: a row holds one source frame, an image-edit instruction for the teacher, and a video-edit instruction for the student.
Offline distillation and \methodname train on the same source rows, and offline training additionally uses the teacher edits described below.
\Cref{fig:training_data} shows how we build a new-task example.

\begin{figure*}[t]
\centering
\includegraphics[width=\textwidth]{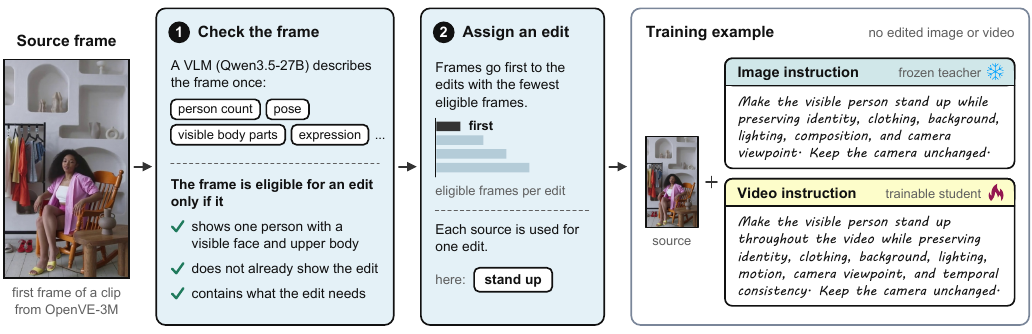}
\caption{\textbf{A new-task training example from \datasetfull.} We check a source frame before assigning it a body-movement edit and then pair it with instructions for the image and video editors.}
\label{fig:training_data}
\end{figure*}

\begin{table}[!htb]
\centering
\fontsize{8}{11}\selectfont
\setlength{\tabcolsep}{1.6pt}
\begin{tabular*}{\linewidth}{@{\extracolsep{\fill}}>{\hspace{2pt}}lr<{\hspace{2pt}}@{}}
\tablehead[l]{Pool and subset} & \tablehead{Source images} \\
\tabheadrule
\textbf{OpenVE pool} & \textbf{6{,}026} \\
\quad \textit{Global Style} & 2{,}000 \\
\quad \textit{Creative Edit} & 1{,}326 \\
\quad \textit{Background Change} & 1{,}000 \\
\quad \textit{Local Add} & 500 \\
\quad \textit{Local Change} & 500 \\
\quad \textit{Local Remove} & 500 \\
\quad \textit{Subtitle Edit} & 200 \\
\tabbodyrule
\textbf{\benchname pool} & \textbf{11{,}201} \\
\quad \textit{Action Change} & 4{,}351 \\
\quad \textit{Expression Change} & 2{,}955 \\
\quad \textit{Body Movement} & 1{,}305 \\
\quad \textit{Scene Relighting} & 2{,}590 \\
\tabbodyrule
\textbf{Total (\datasetfull)} & \textbf{17{,}227} \\
\end{tabular*}
\caption{\textbf{Training pools.} Each source image comes with an image-edit and a video-edit instruction. Counts are from the released data.}
\label{tab:pools}
\end{table}

\paragraph{Source Frames.}
Every source frame is the first frame of a clip from OpenVE-3M~\citep{he2025openve}, at the clip's resolution (mostly $1280\times720$).
The videos are distributed as a split archive, so we take frames by streaming the archive and decoding each clip's first frame in memory.
Before building a pool, we place every clip already used by an earlier pool, by OpenVE-Bench, or by \benchname on an exclusion list. We use each remaining clip at most once within a pool, so no source appears under two instructions.

\paragraph{\benchname Pool.}
\label{app:data_pools}
The \benchname pool covers the four new task groups. We build its action, expression, and body-movement data in four stages.
(1) We extract frames from clips not on the exclusion list.
(2) A VLM (Qwen3.5-27B~\citep{qwen2026qwen35}) describes each frame once, including the people in shot and their pose, gaze, expression, and visible arms.
(3) A frame is eligible for an edit if it shows one person with a visible face and upper body, does not already show the edit, and contains what the edit needs, such as the arm to be raised.
(4) We assign frames to the edits with the fewest eligible frames first to balance the pool.
We state directions in frame terms (``the arm on the left side of the frame''), because ``turn to the left'' leaves open whose left is meant and the teacher resolved it inconsistently.
The data cover 15 action and expression edits and five body-movement edits. We leave out turning to face the camera, for which only three frames were eligible.

The relighting data of the \benchname pool ($2{,}590$ images) ask for a scene light, such as window sunlight, or a colored light, from one of up to ten directions, including front and back light. Most of the 35 light types in the \textit{Scene Relighting} group of \benchname also appear in training.
For most frames, the VLM first classifies the scene (indoor or outdoor, whether a window, water, or street is in shot, and the current light). We then assign only lights that are plausible for the scene and would change the image, so window sunlight goes only to indoor scenes with a window.
The student's instruction ends with a clause asking to preserve the scene content, motion, and camera, whereas the teacher's instruction omits motion.

\paragraph{OpenVE Pool.}
The OpenVE pool takes 6{,}026 source frames from the OpenVE-3M training split in seven categories (\Cref{tab:pools}). For the six categories that the training split covers, it keeps each clip's original instruction as the student's video-edit instruction.
The training split has no \textit{Creative Edit} category, so we build its 1{,}326 rows with the same pipeline as the \benchname pool: a VLM describes each frame and proposes a creative edit that suits it, written as separate instructions for the teacher and the student.

\begin{figure}[!hb]
\centering
\includegraphics[width=\linewidth]{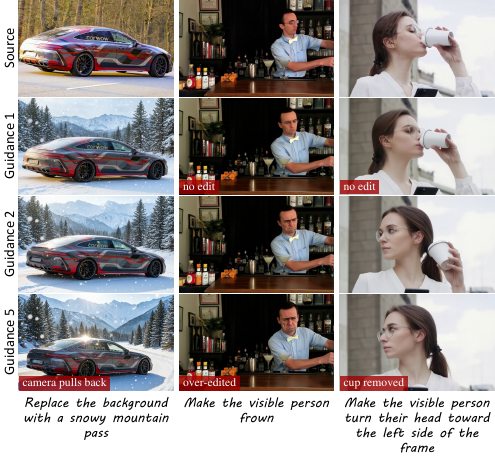}
\caption{\textbf{Teacher guidance for offline distillation targets.} JoyAI-Image-Edit edits training frames at guidance $1$, $2$, and $5$. Instructions are abridged.}
\label{fig:teacher_cfg}
\end{figure}

\paragraph{Teacher Edits for Offline Distillation.}
\label{app:data_targets}
The teacher renders one edit per source image with $50$ sampling steps and guidance $2$ for every offline baseline.
We chose guidance $2$ after rendering training frames at guidance $1$, $2$, and $5$ with the same $50$ steps (\Cref{fig:teacher_cfg}). At guidance $1$, the teacher can leave an edit undone, such as a requested frown or head turn. At guidance $5$, it over-edits by exaggerating expressions, removing objects the instruction does not mention, or moving the camera in background changes. Guidance $2$ is a compromise between these two failure modes and gives stable edits, completing all three examples in \Cref{fig:teacher_cfg} without these side effects.
The teacher resizes its input to a fixed aspect bucket and center-crops what does not fit, so we crop the source to that bucket first and train the student against the cropped source, which keeps source and target aligned.

\section{Additional OpenVE-Bench Results}
\label{app:full_scores}

\Cref{tab:app_full_openve} adds \textit{Creative Edit} and \textit{Subtitle Edit} to the five edit types in \Cref{tab:main} for the same checkpoints and reports the mean over the seven categories.

\begin{table}[!htb]
\centering
\fontsize{8}{9.5}\selectfont
\renewcommand{\deltasize}{\fontsize{4.5}{5.5}\selectfont}
\setlength{\tabcolsep}{0.8pt}
\begin{tabular*}{\linewidth}{@{\extracolsep{\fill}}>{\hspace{2pt}}lccc<{\hspace{2pt}}@{}}
\tablehead{Model} & \tablehead{Creative\\Edit} & \tablehead{Subtitle\\Edit} & \tablehead{7-category\\Overall} \\
\tabheadrule
Bernini-R-1.3B & \scoreonly{3.52} & \scoreonly{3.05} & \scoreonly{3.15} \\
\modelsmall & \scoredelta{3.59}{+0.07} & \scoredelta{3.05}{0.00} & \scoredelta{3.39}{+0.24} \\
\tabbodyrule
Bernini-R-14B & \scoreonly{3.58} & \scoreonly{3.13} & \scoreonly{3.34} \\
\modellarge & \scoredelta{3.61}{+0.03} & \scoredelta{3.17}{+0.04} & \scoredelta{3.53}{+0.19} \\
\tabbodyrule
VideoCoF & \scoreonly{2.32} & \scoreonly{2.67} & \scoreonly{2.35} \\
\modelcof & \scoredelta{3.06}{+0.74} & \scoredelta{3.02}{+0.35} & \scoredelta{3.10}{+0.75} \\
\end{tabular*}
\caption{\textbf{Additional OpenVE-Bench results.} \methodname raises the seven-category score of all three editors, and VideoCoF gains in both added categories. Overall averages the seven categories.}
\label{tab:app_full_openve}
\end{table}

\section{Generalization to IVEBench}
\label{app:ivebench}
We test whether the gains carry over to IVEBench~\citep{chen2026ivebench}, whose clips, instructions, and metrics differ from those of OpenVE-Bench. As in \Cref{sec:ivebench}, we evaluate the jointly trained \modelsmall, \modellarge, and \modelcof on its short-video subset.
\textbf{\methodname achieves state-of-the-art results on IVEBench} (\Cref{tab:ivebench_board}). On the short subset, \modellarge ranks first overall and in instruction compliance among the editors on the \href{https://ryanchenyn.github.io/projects/IVEBench/}{official leaderboard} and AVE~\citep{wang2026ave}.
The overall score averages video quality, instruction compliance, and fidelity, so editors with weak compliance can still score close to the top. Ditto, for example, scores $66.7$ on IVEBench, close to \modelsmall ($68.9$), but $2.13$ on OpenVE-Bench against $3.42$ (\Cref{tab:main}).
IVEBench computes video quality from four temporal consistency metrics and a single-frame aesthetic score (\Cref{tab:ivebench_main}).

\begin{table}[!htb]
\centering
\fontsize{8}{9.5}\selectfont
\setlength{\tabcolsep}{1.6pt}
\begin{tabular*}{\linewidth}{@{\extracolsep{\fill}}>{\hspace{2pt}}lcccc<{\hspace{2pt}}@{}}
\tablehead[l]{Method} & \tablehead{Overall$^{\uparrow}$} & \tablehead{Video\\Quality$^{\uparrow}$} & \tablehead{Instruction\\Compliance$^{\uparrow}$} & \tablehead{Fidelity$^{\uparrow}$} \\
\tabheadrule
\shadedrow
\modellarge & \textbf{71.5} & 78.4 & \textbf{56.0} & 80.3 \\
Bernini-R-14B$^\star$ & 71.0 & 78.7 & 53.7 & 80.3 \\
AVE$^\dagger$~\citep{wang2026ave} & 70.6 & \textbf{82.1} & 49.7 & 80.0 \\
\shadedrow
\modelsmall & 68.9 & 79.1 & 50.5 & 77.1 \\
\shadedrow
\modelcof & 68.2 & 80.6 & 40.5 & \textbf{83.5} \\
Bernini-R-1.3B$^\star$ & 67.4 & 79.3 & 42.8 & 80.2 \\
Ditto~\citep{bai2026ditto} & 66.7 & 78.1 & 49.1 & 73.0 \\
InsV2V~\citep{cheng2024insv2v} & 66.7 & 79.6 & 38.6 & 81.9 \\
Lucy-Edit-Dev~\citep{decart2025lucyedit} & 63.5 & \textbf{82.1} & 33.9 & 74.6 \\
VACE~\citep{jiang2025vace} & 62.6 & 79.8 & 25.4 & 82.6 \\
ICVE~\citep{liao2025icve} & 60.3 & 71.3 & 45.4 & 64.4 \\
Omni-Video~\citep{tan2026omnivideo} & 58.7 & 78.2 & 43.6 & 54.1 \\
AnyV2V~\citep{ku2024anyv2v} & 57.7 & 72.7 & 41.7 & 58.6 \\
VideoCoF$^\star$~\citep{yang2025videocof} & 52.9 & 71.4 & 25.5 & 61.6 \\
StableV2V & 50.9 & 69.2 & 42.7 & 40.8 \\
\end{tabular*}
\caption{\textbf{IVEBench short-subset leaderboard.} \modellarge ranks first overall. Unmarked rows are from the official leaderboard, the row marked $\dagger$ is from its paper, and we evaluate the rows marked $\star$ and our models. Scores $\times100$.}
\label{tab:ivebench_board}
\end{table}


\section{More Ablations}
\label{app:ablation}

We report the five-category OpenVE-Bench score for the following OpenVE-pool comparisons.
\subsection{Rollout Schedule}
\Cref{tab:ablation_schedule} varies the number of rollout steps $K$ and the rollout time shift of Bernini-R-1.3B on the OpenVE pool, one at a time from the default ($K=10$, time shift $5$).
\textbf{Shorter rollouts lower the score}: with 8 or 5 steps, Overall drops from $3.48$ to $3.33$ or $3.39$. A time shift of $3$ scores slightly higher ($3.54$), and a shift of $1$ scores $3.36$.

\begin{table}[!hb]
\centering
\fontsize{8}{9.5}\selectfont
\renewcommand{\deltasize}{\fontsize{4.5}{5.5}\selectfont}
\setlength{\tabcolsep}{1.6pt}
\begin{tabular*}{\linewidth}{@{\extracolsep{\fill}}>{\hspace{2pt}}lcccccc<{\hspace{2pt}}@{}}
\tablehead{Setting} & \tablehead{Global\\Style$^{\uparrow}$} & \tablehead{Local\\Change$^{\uparrow}$} & \tablehead{Background\\Change$^{\uparrow}$} & \tablehead{Local\\Remove$^{\uparrow}$} & \tablehead{Local\\Add$^{\uparrow}$} & \tablehead{Overall$^{\uparrow}$} \\
\tabheadrule
Base & \scoreonly{3.27} & \scoreonly{4.01} & \scoreonly{2.94} & \scoreonly{2.88} & \scoreonly{2.41} & \scoreonly{3.10} \\
\shadedrow
Default & \scoredelta{\textbf{4.04}}{+0.77} & \scoredelta{4.21}{+0.20} & \scoredelta{3.03}{+0.09} & \scoredelta{\textbf{3.50}}{+0.62} & \scoredelta{2.61}{+0.20} & \scoredelta{3.48}{+0.38} \\
\tabbodyrule
$K=8$ & \scoredelta{3.91}{+0.64} & \scoredelta{4.13}{+0.12} & \scoredelta{2.98}{+0.04} & \scoredelta{3.09}{+0.21} & \scoredelta{2.52}{+0.11} & \scoredelta{3.33}{+0.23} \\
$K=5$ & \scoredelta{4.01}{+0.74} & \scoredelta{4.01}{0.00} & \scoredelta{3.01}{+0.07} & \scoredelta{3.39}{+0.51} & \scoredelta{2.50}{+0.09} & \scoredelta{3.39}{+0.29} \\
\tabbodyrule
Shift $3$ & \scoredelta{4.03}{+0.76} & \scoredelta{\textbf{4.33}}{+0.32} & \scoredelta{\textbf{3.19}}{+0.25} & \scoredelta{3.48}{+0.60} & \scoredelta{\textbf{2.70}}{+0.29} & \scoredelta{\textbf{3.54}}{+0.44} \\
Shift $1$ & \scoredelta{3.84}{+0.57} & \scoredelta{4.16}{+0.15} & \scoredelta{2.81}{-0.13} & \scoredelta{3.42}{+0.54} & \scoredelta{2.57}{+0.16} & \scoredelta{3.36}{+0.26} \\
\end{tabular*}
\caption{\textbf{Ablation on the rollout schedule.} Shorter rollouts lower the score, and a time shift of $3$ scores slightly above the default of $5$. Bernini-R-1.3B trained on the OpenVE pool.}
\label{tab:ablation_schedule}
\end{table}

\subsection{Matching Losses}
\label{app:loss}

We compare mse and cos losses on velocity predictions ($\vv$) and predicted clean latents ($\vx$), using Bernini-R-1.3B on the OpenVE pool with $\omega_R=\omega_S=\omega_T=1$, and report the five-category comparison in \Cref{tab:abl_loss}.

Writing $\vv^S_k$ and $\vv^T_k$ for the student and teacher velocities in \cref{eq:loss}, at the same rollout state $\vx_{t_k}$ the student and teacher predict clean latents as
\begin{equation}
\begin{gathered}
\hat{\vx}^S_{0,k} = \vx_{t_k}-t_k \vv^S_k, \\
\hat{\vx}^T_{0,k} = \sg(\vx_{t_k}-t_k \vv^T_k).
\end{gathered}
\label{eq:abl_clean_predictions}
\end{equation}

We apply either distance below to the velocity pair $(\vv^S_k,\sg(\vv^T_k))$ or the clean-latent pair $(\hat{\vx}^S_{0,k},\hat{\vx}^T_{0,k})$:
\begin{equation}
\begin{gathered}
\ell_{\mathrm{mse}}(a,b)
  = \frac{1}{NC}\sum_{j=1}^{N}\lVert a_j-b_j\rVert_2^2, \\
\ell_{\mathrm{cos}}(a,b)
  = \frac{1}{N}\sum_{j=1}^{N}\left(1-
  \frac{\langle a_j,b_j\rangle}{\lVert a_j\rVert_2\lVert b_j\rVert_2}\right).
\end{gathered}
\label{eq:abl_matching_distances}
\end{equation}
Here $N$ is the number of latent positions and $C$ the channel dimension, with losses averaged over rollout states as in \cref{eq:loss}.

Because the two predictions share the state $\vx_{t_k}$, the clean-latent difference equals $-t_k$ times the velocity difference. A change of loss space thus effectively reweights the loss~\citep{li2025jit}: the clean-latent mse is a reweighted form of the velocity mse, with weight $t_k^2$ at step $k$. The comparison between $v$ and $x$ therefore changes both the matched quantity and the weighting across rollout steps.

\section{\benchname}
\label{app:extended}

\benchname contains 207 clips in four groups: \textit{Action Change} (73 clips with head, gaze, and arm edits), \textit{Expression Change} (42), \textit{Body Movement} (42), and \textit{Scene Relighting} (50, with 35 light types and 10 directions, phrased differently from the training data). Overall is the mean of the four group means.
The source clips come from OpenVE-3M videos that no training pool uses, so \benchname follows the CC BY-NC 4.0 license of OpenVE-3M.
For the action, expression, and body-movement groups, a VLM checks that the first frame suits the edit, and we check that the requested change does not already appear later in the clip.
For relighting, Qwen3.5-27B~\citep{qwen2026qwen35} checks that the requested light would visibly change the clip, that the clip is not already lit that way, and that the light fits the scene. Finally, we check every case of the four groups by hand.
\Cref{fig:openvepp} shows edits of Bernini-R-1.3B on \benchname.

\begin{figure*}[t]
\centering
\includegraphics[width=\linewidth]{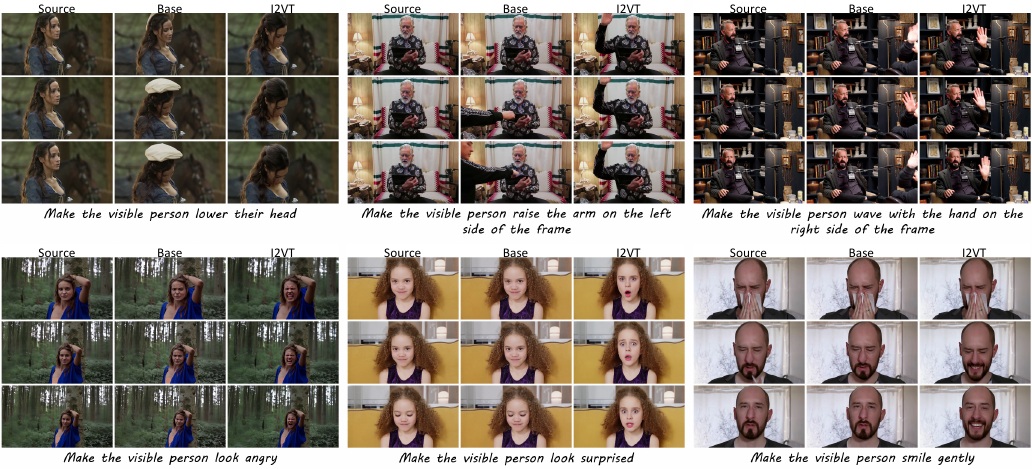}
\caption{\textbf{New abilities on \benchname} (Bernini-R-1.3B). Each example shows three frames of the source, the base editor, and the student trained with \methodname. Asked to lower the woman's head (top left), the base editor adds a cap, and asked to raise the man's arm (top middle), it adds another person's arm.}
\label{fig:openvepp}
\end{figure*}


\begin{table}[!hb]
\centering
\newcommand{\cmark}{\textcolor{ForestGreen}{\ensuremath{\checkmark}}}
\newcommand{\pmark}{\textcolor{gray}{\ensuremath{\circ}}}
\newcommand{\xmark}{\textcolor{BrickRed}{\ensuremath{\times}}}
\fontsize{8}{9.5}\selectfont
\setlength{\tabcolsep}{1.6pt}
\begin{tabular*}{\linewidth}{@{\extracolsep{\fill}}>{\hspace{2pt}}lcccc<{\hspace{2pt}}@{}}
 & \tablehead{IVEBench} & \tablehead{CoVE-\\Bench} & \tablehead{Goku-\\Bench} & \tablehead{\benchname} \\
\tabheadrule
Action Change      & \pmark & \pmark & \pmark & \cmark \\
Expression Change  & \pmark & \pmark & \xmark & \cmark \\
Body Movement      & \cmark & \pmark & \cmark & \cmark \\
Scene Relighting   & \xmark & \xmark & \xmark & \cmark \\
Single Edit        & \cmark & \pmark & \xmark & \cmark \\
Open Source        & \cmark & \cmark & \xmark & \cmark \\
\end{tabular*}
\caption{\textbf{\benchname and other video editing benchmarks.} \cmark: a dedicated category. \pmark: a few cases in a broader category. \xmark: no coverage.}
\label{tab:bench_compare}
\end{table}

\paragraph{Comparison with Other Benchmarks.}
\Cref{tab:bench_compare} compares \benchname with three recent benchmarks. \emph{Single Edit} means that each instruction asks for one edit, and \emph{Open Source} means that the test set is public. \benchname will be released with the paper.
IVEBench~\citep{chen2026ivebench} puts motion edits, including six laughing or crying edits, into one \textit{Subject Motion Editing} category and has no lighting edits.
CoVEBench~\citep{wu2026covebench} covers expressions, actions, and lighting changes, but 583 of its 626 instructions combine several edits, so its marks in \Cref{tab:bench_compare} count only the 43 single-edit instructions. None of its lighting edits specifies a light type and direction.
Goku-Bench~\citep{liang2026goku} has a \textit{Subject Movement} category without expression or lighting edits, and its test set has not been released.
\benchname gives each of the four task groups its own category and asks for one edit per instruction, so each group score measures one ability.

\section{User Study}
\label{app:user_study}

We run a user study to check whether people also prefer \methodname edits over those of the base editors on \benchname.
For each of the four task groups, we select four \benchname clips and compare two pairs of editors from \Cref{tab:main}: Bernini-R-1.3B with \modelsmall, and Bernini-R-14B with \modellarge.
Each of 20 participants judges 16 pairs of edits, two clips per task group for each editor pair. For every pair, a participant chooses which edit is better overall or calls a tie, without separate criteria.
The participants are volunteers recruited from the authors' acquaintances, and we record only their choices, with no names, contact details, or other personal data. No IRB or equivalent body reviewed the study, since it studies nothing about the participants themselves, and the participants agreed to take part without a written consent form.

\begin{table}[t]
\centering
\fontsize{8}{9.5}\selectfont
\setlength{\tabcolsep}{1.6pt}
\begin{tabular*}{\linewidth}{@{\extracolsep{\fill}}>{\hspace{2pt}}lcccccc<{\hspace{2pt}}@{}}
 & \multicolumn{3}{c}{\tablehead{\modelsmall vs.\ Base}} & \multicolumn{3}{c}{\tablehead{\modellarge vs.\ Base}} \\
\tabgrouprule{2-4}\tabgrouprule{5-7}
\tablehead[l]{Task group} & \tablehead{Win$^{\uparrow}$} & \tablehead{Tie} & \tablehead{Loss$^{\downarrow}$} & \tablehead{Win$^{\uparrow}$} & \tablehead{Tie} & \tablehead{Loss$^{\downarrow}$} \\
\tabheadrule
Action Change & 72.5 & 20.0 & 7.5 & 50.0 & 30.0 & 20.0 \\
Expression Change & 60.0 & 27.5 & 12.5 & 62.5 & 22.5 & 15.0 \\
Body Movement & 62.5 & 37.5 & 0.0 & 35.0 & 50.0 & 15.0 \\
Scene Relighting & 77.5 & 15.0 & 7.5 & 55.0 & 35.0 & 10.0 \\
\tabbodyrule
All & 68.1 & 25.0 & 6.9 & 50.6 & 34.4 & 15.0 \\
\end{tabular*}
\caption{\textbf{User study on \benchname.} Participants prefer \methodname over the base editor in every task group. Each cell is the percentage of the 40 judgments (160 in the last row) in which \methodname wins, ties, or loses.}
\label{tab:user_study}
\end{table}

\textbf{Participants prefer \methodname over the base editor in every task group at both sizes} (\Cref{tab:user_study}).
\modelsmall wins 68.1\% of its 160 judgments and loses 6.9\%. Against the stronger Bernini-R-14B, \modellarge wins 50.6\% and loses 15.0\%, and more of its judgments end in a tie, most of all for body movements (50.0\%).
This preference agrees in direction with the Gemini 2.5 Pro scores on \benchname in \Cref{tab:main}.

\section{Evaluation Details}
\label{app:evaluation_protocol}

We follow the OpenVE-Bench protocol~\citep{he2025openve}, whose authors report close agreement with human judgment. For each edit, the Gemini judge receives the source video followed by the edited video as two video-file inputs, with a category-specific scoring prompt supplied as the system instruction. We upload the complete videos without local frame extraction and leave the temperature at the API default for the Gemini 2.5 Pro runs.

The prompts, including those for \benchname in Appendix~\ref{app:eval_prompts}, rate instruction compliance, consistency with the source, and visual quality from 1 to 5~\citep{ku2024viescore,zheng2023judging}. They penalize flickering and other temporal artifacts according to the category-specific rubric, and instruct the evaluator not to assign consistency or quality scores above instruction compliance. We average the three ratings for each clip, then average clip scores within each category and category means for Overall.

For comparisons with published editors, we report five OpenVE-Bench categories: \textit{Global Style}, \textit{Local Change}, \textit{Background Change}, \textit{Local Remove}, and \textit{Local Add}, following the five-category comparison of prior work such as Kiwi-Edit~\citep{lin2026kiwiedit} and JoyAI-Video-Edit~\citep{xiao2026joyaivideoedit}.

\paragraph{Published OpenVE-Bench Scores.}
\label{app:published_scores}
For the unmarked rows of existing editors in \Cref{tab:main}, we take VACE, OpenVE-Edit, ICVE, Ditto, and Lucy-Edit scores from the OpenVE-3M table ``Quantitative Comparison on OpenVE-Bench with Gemini 2.5 Pro'' (Table~3 of arXiv v2)~\citep{he2025openve}, and Kiwi-Edit scores from Table~2 of Kiwi-Edit~\citep{lin2026kiwiedit}. VInO scores come from its Table~7~\citep{chen2026vino} and LoomVideo scores from its OpenVE-Bench comparison~\citep{loomvideo2026}. We count VInO as 17B, its 13B HunyuanVideo generation backbone plus its Qwen3-VL-4B encoder~\citep{chen2026vino}.
We map columns by category name and recompute Overall as the mean of the five reported categories.
We evaluate the starred rows (Bernini-R-1.3B, VideoCoF, Bernini-R-14B, and JoyAI-Video-Edit) with this OpenVE-Bench protocol, running each with the default inference settings of its official repository.

\paragraph{\benchname Scores from a Second Judge.}
\label{app:second_judge}

\Cref{tab:flash} lists the Gemini 3.8 Flash scores from \Cref{tab:main}. We used the same prompts (\Cref{app:eval_prompts}) and aggregation for both judges. OpenVE-Edit has no results on \benchname because its weights are unavailable.

\begin{table}[t]
\centering
\fontsize{8}{9.5}\selectfont
\setlength{\tabcolsep}{0.5pt}
\begin{tabular*}{\linewidth}{@{\extracolsep{\fill}}>{\hspace{2pt}}lccccc<{\hspace{2pt}}@{}}
\tablehead[l]{Model} & \tablehead{Action\\Change$^{\uparrow}$} & \tablehead{Expression\\Change$^{\uparrow}$} & \tablehead{Body\\Movement$^{\uparrow}$} & \tablehead{Scene\\Relighting$^{\uparrow}$} & \tablehead{Overall$^{\uparrow}$} \\
\tabheadrule
Bernini-R-1.3B & 1.43 & 1.50 & 1.10 & 2.11 & 1.54 \\
Lucy-Edit & 1.34 & 1.51 & 1.04 & 2.07 & 1.49 \\
Kiwi-Edit & 1.11 & 1.97 & 1.00 & 2.43 & 1.63 \\
LoomVideo (RL) & 1.26 & 1.40 & 1.30 & 3.10 & 1.77 \\
ICVE & 1.24 & 1.56 & 1.07 & 1.98 & 1.46 \\
VACE & 1.10 & 1.36 & 1.00 & 2.77 & 1.56 \\
Ditto & 1.68 & 2.79 & 1.00 & 3.03 & 2.13 \\
VideoCoF & 1.11 & 1.12 & 1.00 & 1.41 & 1.16 \\
Bernini-R-14B & 2.57 & 1.31 & 2.47 & 2.84 & 2.30 \\
JoyAI-Video-Edit & 2.51 & 2.21 & 2.52 & 3.76 & 2.75 \\
VInO & 3.29 & 3.94 & 2.45 & 3.55 & 3.31 \\
\tabbodyrule
\shadedrow
\modelsmall & 3.35 & 3.67 & 2.90 & 3.65 & 3.39 \\
\shadedrow
\modellarge & 3.86 & 3.82 & \textbf{3.67} & 3.73 & 3.77 \\
\shadedrow
\modelcof & \textbf{4.07} & \textbf{4.53} & 3.14 & \textbf{4.27} & \textbf{4.01} \\
\end{tabular*}
\caption{\textbf{\benchname scores from Gemini 3.8 Flash.} The three \methodname models still score highest overall, and each improves on its base editor in every task group.}
\label{tab:flash}
\end{table}

\textbf{The two judges give similar Overall rankings on \benchname} (\Cref{tab:main}).
Under Gemini 3.8 Flash, \modelcof, \modellarge, and \modelsmall take the top three Overall scores ($4.01$, $3.77$, and $3.39$), and each improves on its base editor in all four task groups.
Spearman's $\rho$ is $0.91$ across the 14 editors with scores from both judges.

\section{Evaluation Prompts}
\label{app:eval_prompts}
OpenVE-Bench uses the scoring prompts released with OpenVE-3M~\citep{he2025openve}. Below are the prompts for the four \benchname groups, written in the same three-axis format. The placeholder \texttt{\{edit\_prompt\}} is replaced by the requested editing instruction, and the source and edited videos are supplied in that order.

\begin{promptbox}{Evaluation Prompt of Action Change}
You are a data rater specializing in grading video edits that change a visible person's pose, gesture, facial expression, or gaze while preserving the camera.\par
\textbf{Instruction Compliance}\par
1. The requested action is absent, targets the wrong subject, changes the camera, or makes an unrelated edit.\par
2. The requested action is weakly attempted, changes the wrong body part/expression, or introduces camera movement.\par
3. The action is recognizable but inaccurate in direction, degree, limb, expression, or consistency.\par
4. The requested action is correct with only minor pose, anatomy, expression, or temporal inaccuracies.\par
5. The requested action is executed precisely and consistently while keeping the camera unchanged.\par
\textbf{Visual Quality \& Stability}\par
1. Severe artifacts, broken anatomy, unusable face/hands, flicker, or major video corruption.\par
2. Obvious anatomical distortions, face damage, jitter, or distracting artifacts.\par
3. Acceptable but with visible local artifacts, imperfect anatomy, or temporal instability.\par
4. Clean and stable result with only minor artifacts.\par
5. Natural, clean, realistic, and temporally stable action edit.\par
\textbf{Consistency \& Detail Fidelity}\par
1. Background, identity, clothing, camera viewpoint, or unrelated objects are heavily changed.\par
2. Important unrelated details are changed or the person identity/camera viewpoint is unstable.\par
3. Main content is preserved but with noticeable unintended changes.\par
4. Nearly all unrelated details and camera viewpoint are preserved.\par
5. Only the requested action changes; identity, clothing, background, and camera viewpoint are perfectly preserved.\par
The second and third scores should not be higher than the first score.\par
\textbf{Example Response Format}\par
Brief reasoning: No more than 20 words.\par
Instruction Compliance: 1-5.\par
Visual Quality \& Stability: 1-5.\par
Consistency \& Detail Fidelity: 1-5.\par
Editing instruction is: \{edit\_prompt\}.\par
Below are the videos before and after editing:\par
\end{promptbox}

\begin{promptbox}{Evaluation Prompt of Expression Change}
You are a data rater specializing in grading video edits that change a visible person's facial expression while leaving everything else, including the head pose and the camera, unchanged.\par
\textbf{Instruction Compliance}\par
1. The face is unchanged, or it shows a different emotion than the one asked for, or the edit lands on the wrong person.\par
2. The expression shifts but reads as the wrong emotion, appears on part of the face only, or arrives with a head turn or camera move that was not requested.\par
3. The requested emotion is recognizable but under- or over-played, inconsistent between the mouth and the eyes, or unstable across frames.\par
4. The requested emotion is clearly present and read correctly from both mouth and brow, with minor timing or intensity imperfections.\par
5. The requested emotion is unmistakable, coherent across mouth, brow and eyes, and held steadily for the whole clip.\par
\textbf{Visual Quality \& Stability}\par
1. The face is destroyed: melted features, doubled mouths, broken teeth or eyes, or heavy flicker.\par
2. Obvious facial distortion, unstable features between frames, or distracting artifacts around the mouth and eyes.\par
3. Acceptable but with visible local artifacts on the face or mild frame-to-frame wobble.\par
4. Clean and stable, with only minor imperfections in fine facial detail.\par
5. Natural and photographic throughout, with skin, teeth and eyes rendered convincingly and no flicker.\par
\textbf{Consistency \& Detail Fidelity}\par
1. The person has been replaced, or hair, clothing, background or camera viewpoint are heavily changed.\par
2. Identity drifts noticeably, or the head pose, framing or background changes along with the expression.\par
3. The person remains recognizable but with unintended changes to face shape, hair, or surroundings.\par
4. Identity, head pose, clothing, background and camera viewpoint are nearly all preserved.\par
5. Only the expression changes; the same person, the same head pose, the same clothing, background and camera viewpoint.\par
The second and third scores should not be higher than the first score.\par
\textbf{Example Response Format}\par
Brief reasoning: No more than 20 words.\par
Instruction Compliance: 1-5.\par
Visual Quality \& Stability: 1-5.\par
Consistency \& Detail Fidelity: 1-5.\par
Editing instruction is: \{edit\_prompt\}.\par
Below are the videos before and after editing:\par
\end{promptbox}

\begin{promptbox}{Evaluation Prompt of Body Movement}
You are a data rater specializing in grading video edits that make a visible person perform a whole-body movement -- jumping, crouching, standing up, sitting down, or turning to face the other way -- while the camera stays where it was.\par
\textbf{Instruction Compliance}\par
1. The person does not move, performs a different movement, or the camera moves or cuts instead.\par
2. A movement is attempted but it is the wrong one, only partially carried out, or achieved by zooming, panning or re-framing rather than by the person moving.\par
3. The requested movement is recognizable but incomplete, in the wrong direction, or the body does not follow through the way the instruction implies.\par
4. The requested movement is carried out correctly with minor errors in extent, timing, or balance.\par
5. The requested movement is performed fully and plausibly, with the whole body following through, and the camera unchanged.\par
\textbf{Visual Quality \& Stability}\par
1. Limbs detach, duplicate or melt; the body is unusable or the clip is badly corrupted.\par
2. Obvious anatomical breakage during the movement, or heavy jitter as the pose changes.\par
3. Acceptable but with visible distortion at the joints, feet or hands while moving.\par
4. Clean and stable through the movement with only minor artifacts.\par
5. Anatomically sound and temporally smooth from start to finish.\par
\textbf{Consistency \& Detail Fidelity}\par
1. The person is replaced, or the room, floor, furniture or camera viewpoint are rebuilt around the movement.\par
2. Identity or surroundings change noticeably, or the framing shifts to accommodate the new pose.\par
3. The scene survives but with unintended changes to clothing, nearby objects, or the person's proportions.\par
4. Identity, clothing, background and camera viewpoint are nearly all preserved through the movement.\par
5. Only the person's pose changes; identity, clothing, the surrounding scene and the camera viewpoint are untouched.\par
The second and third scores should not be higher than the first score.\par
\textbf{Example Response Format}\par
Brief reasoning: No more than 20 words.\par
Instruction Compliance: 1-5.\par
Visual Quality \& Stability: 1-5.\par
Consistency \& Detail Fidelity: 1-5.\par
Editing instruction is: \{edit\_prompt\}.\par
Below are the videos before and after editing:\par
\end{promptbox}

\begin{promptbox}{Evaluation Prompt of Scene Relighting}
You are a data rater specializing in grading video relighting edits. You will be given two videos (before and after editing) and the editing instruction.\par
\textbf{Instruction Compliance}\par
1. Lighting is unchanged, changed in the wrong direction/style, or the edit is unrelated.\par
2. The requested lighting appears only weakly, in the wrong area, or with major style mismatch.\par
3. The requested lighting is recognizable but incomplete, inconsistent, or mixed with incorrect illumination.\par
4. The requested lighting is applied well with only minor intensity, direction, or color inaccuracies.\par
5. The lighting exactly matches the requested style and direction while preserving the original scene content.\par
\textbf{Visual Quality \& Stability}\par
1. Severe flicker, artifacts, blown-out regions, or unusable video.\par
2. Distracting temporal instability, inconsistent shadows, or obvious relighting artifacts.\par
3. Mostly stable but with visible lighting flicker, halos, or local artifacts.\par
4. Stable and clean relighting with only minor artifacts.\par
5. Perfectly stable, natural illumination, shadows, and color across the whole video.\par
\textbf{Consistency \& Detail Fidelity}\par
1. Objects, identity, materials, motion, or camera viewpoint are heavily changed.\par
2. Important scene details or geometry are changed while relighting.\par
3. Main content is preserved but with noticeable unintended changes.\par
4. Nearly all unrelated details, motion, and camera viewpoint are preserved.\par
5. Only lighting changes; all scene content, motion, materials, and camera viewpoint are perfectly preserved.\par
The second and third scores should not be higher than the first score.\par
\textbf{Example Response Format}\par
Brief reasoning: No more than 20 words.\par
Instruction Compliance: 1-5.\par
Visual Quality \& Stability: 1-5.\par
Consistency \& Detail Fidelity: 1-5.\par
Editing instruction is: \{edit\_prompt\}.\par
Below are the videos before and after editing:\par
\end{promptbox}


\section{Additional VideoCoF Results}
\label{app:videocof_gallery}

\Cref{fig:videocof_gallery} shows edits from \modelcof on OpenVE-Bench and \benchname.

\begin{figure*}[t]
\centering
\includegraphics[width=\linewidth]{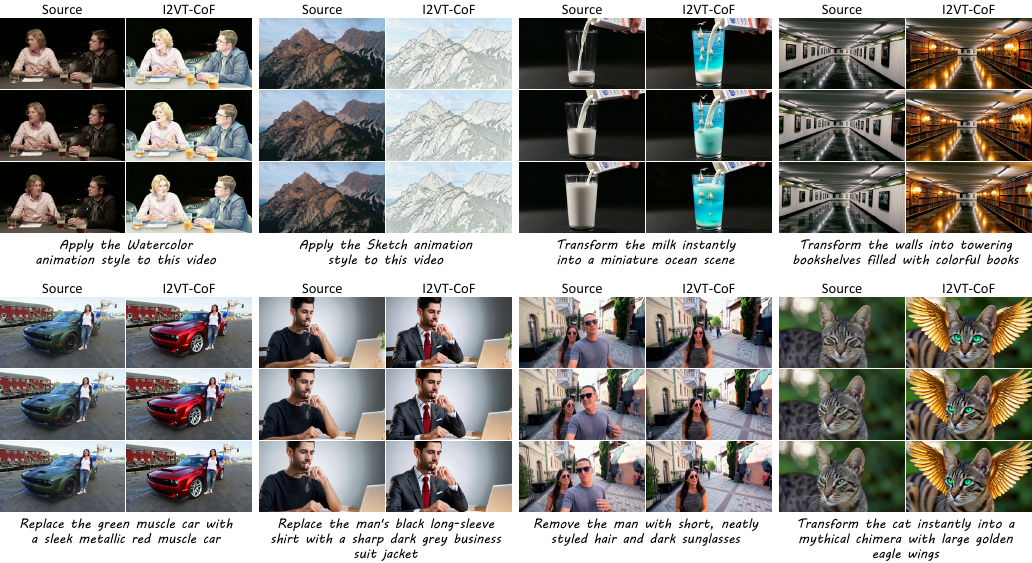}
\\[3pt]
\includegraphics[width=\linewidth]{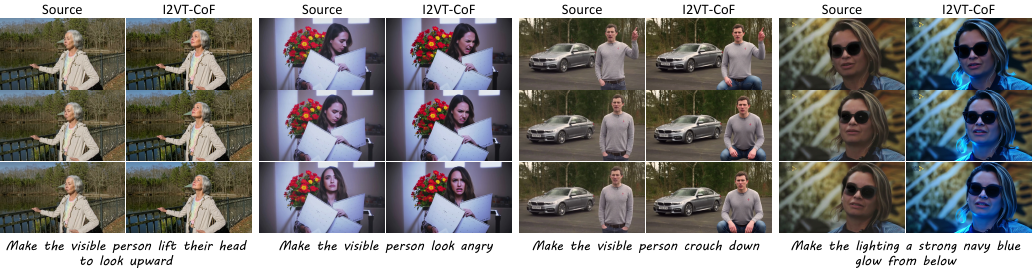}
\caption{\textbf{\modelcof on OpenVE-Bench and \benchname.} Each example shows three source frames (left) and the edited frames (right). The bottom row shows one \benchname edit from each new task group. Instructions are abridged.}
\label{fig:videocof_gallery}
\end{figure*}
